# Supplementary material for: Model-agnostic and Scalable Counterfactual Explanations via Reinforcement Learning
Source: arXiv:2106.02597 source file (2021-06-04)
Supplement: Supplementary file 1 [file 09-soft_targets.tex]

\clearpage
\section{Significance}

\begin{table*}[!htbp]
  \caption{Comparison validity, absolute distance to target (0.75), sparsity, and in-distributioness (unbalanced dataset, untrained encoder)}
  \label{tab:comparison_significance}
  \centering
  
  \begin{tabular}{llllllllll}
    \toprule
    &               \multicolumn{7}{c}{\textbf{Metrics}} \\
                    \cmidrule(r){2-8} 
    \textbf{Method}            &\textbf{Validity}(\%)   &\textbf{Abs. dist. (valid)}    &\textbf{Abs. dist. (all)} &\boldsymbol{$L_{0}$}  &\boldsymbol{$L_{1}$}  &\boldsymbol{$MMD_{0}$}  &\boldsymbol{$MMD_{1}$} \\
    s=0.5, c=0.5, b=1.0        &$86.76 + 17.81$	         &$0.12 + 0.06$	                &$0.17 + 0.13$	        &$0.25 + 0.15$	       &$0.18 + 0.09$		      &$0.28 + 0.25$	  &$0.36 + 0.30$ \\
    s=0.5, c=0.5, b=0.5        &$89.65 + 13.32$	         &$0.13 + 0.05$	                &$0.17 + 0.10$	        &$0.25 + 0.15$	       &$0.19 + 0.10$		      &$0.29 + 0.24$	  &$0.35 + 0.28$ \\
    s=0.4, c=0.5, b=0.5        &$92.78 + 10.07$	         &$0.13 + 0.05$	                &$0.16 + 0.09$	        &$0.27 + 0.16$	       &$0.20 + 0.11$		      &$0.30 + 0.25$	  &$0.40 + 0.37$ \\
    s=0.3, c=0.5, b=0.5        &$94.80 + 6.55$	         &$0.12 + 0.06$	                &$0.14 + 0.07$	        &$0.30 + 0.17$	       &$0.22 + 0.13$		      &$0.29 + 0.25$	  &$0.38 + 0.38$ \\
    \midrule
    s=0.5, c=0.5, b=1.0, cond  &$82.72 + 18.36$	         &$0.12 + 0.06$	                &$0.19 + 0.14$	        &$0.22 + 0.15$	       &$0.19 + 0.08$	          &$0.33 + 0.33$	  &$0.21 + 0.15$ \\
    s=0.5, c=0.5, b=0.5, cond  &$85.38 + 15.20$	         &$0.14 + 0.05$	                &$0.19 + 0.12$	        &$0.22 + 0.15$	       &$0.19 + 0.08$	          &$0.33 + 0.31$      &$0.21 + 0.14$ \\
    s=0.4, c=0.5, b=0.5, cond  &$87.33 + 14.08$	         &$0.13 + 0.05$	                &$0.18 + 0.11$	        &$0.25 + 0.16$	       &$0.21 + 0.09$	          &$0.33 + 0.32$	  &$0.20 + 0.16$ \\
    s=0.3, c=0.5, b=0.5, cond  &$89.89 + 10.62$	         &$0.13 + 0.06$	                &$0.17 + 0.09$	        &$0.27 + 0.17$	       &$0.23 + 0.10$	          &$0.31 + 0.29$	  &$0.20 + 0.17$ \\
    \bottomrule
  \end{tabular}
\end{table*}

\begin{table*}[!htbp]
  \caption{Comparison validity, sparsity, in-distributioness for coarse ranges of target (unbalanced dataset, untrained encoder).}
  \label{tab:comparison_soft_targets_coarse}
  \centering
  
  \begin{tabular}{llllllll}
    \toprule
                                &\multicolumn{2}{c}{Prob}         &\multicolumn{5}{c}{\textbf{Metrics}} \\
                               \cmidrule(r){2-3}                  \cmidrule(r){4-8} 
    \textbf{Method}            &\textbf{Min}   &\textbf{Max}      &\textbf{Validity}(\%)  &\boldsymbol{$L_{0}$}  &\boldsymbol{$L_{1}$}  &\boldsymbol{$MMD_{0}$}   &\boldsymbol{$MMD_{1}$} \\
    \midrule
    s=0.3, c=0.5, b=0.5        &$0.50$    &$0.99$	&$88.62 + 6.45$	    &$0.30 + 0.17$	&$0.23 + 0.12$		&$0.26 + 0.25$	&$0.32 + 0.31$	\\
    s=0.3, c=0.5, b=0.5        &$0.60$    &$0.99$	&$94.00 + 5.63$	    &$0.31 + 0.18$	&$0.23 + 0.13$		&$0.25 + 0.24$	&$0.36 + 0.35$    \\
    s=0.3, c=0.5, b=0.5        &$0.70$    &$0.99$	&$96.45 + 4.82$	    &$0.31 + 0.18$	&$0.24 + 0.13$		&$0.25 + 0.23$	&$0.39 + 0.38$    \\
    s=0.3, c=0.5, b=0.5        &$0.80$    &$0.99$	&$97.50 + 4.47$     &$0.32 + 0.18$	&$0.25 + 0.13$		&$0.24 + 0.23$	&$0.42 + 0.41$    \\
    s=0.3, c=0.5, b=0.5        &$0.90$    &$0.99$	&$97.84 + 4.42$	    &$0.32 + 0.19$	&$0.26 + 0.13$		&$0.23 + 0.23$	&$0.44 + 0.44$    \\
    s=0.3, c=0.5, b=0.5        &$0.99$    &$0.99$	&$98.05 + 4.36$	    &$0.32 + 0.19$	&$0.27 + 0.13$		&$0.23 + 0.23$	&$0.45 + 0.44$    \\
    \midrule
    s=0.4, c=0.5, b=0.5        &$0.50$    &$0.99$	&$86.11 + 9.51$	    &$0.27 + 0.16$	&$0.20 + 0.10$		&$0.28 + 0.25$	&$0.34 + 0.31$    \\
    s=0.4, c=0.5, b=0.5        &$0.60$    &$0.99$	&$92.10 + 9.43$	    &$0.27 + 0.17$	&$0.21 + 0.11$		&$0.27 + 0.25$	&$0.38 + 0.35$    \\
    s=0.4, c=0.5, b=0.5        &$0.70$    &$0.99$	&$94.70 + 9.31$	    &$0.28 + 0.17$	&$0.22 + 0.11$		&$0.26 + 0.25$	&$0.40 + 0.37$    \\
    s=0.4, c=0.5, b=0.5        &$0.80$    &$0.99$	&$95.79 + 9.18$	    &$0.28 + 0.17$	&$0.23 + 0.11$		&$0.26 + 0.25$	&$0.42 + 0.38$    \\
    s=0.4, c=0.5, b=0.5        &$0.90$    &$0.99$	&$96.15 + 9.07$	    &$0.29 + 0.18$	&$0.23 + 0.11$		&$0.25 + 0.24$	&$0.43 + 0.39$    \\
    s=0.4, c=0.5, b=0.5        &$0.99$    &$0.99$	&$96.37 + 8.89$	    &$0.29 + 0.18$	&$0.24 + 0.11$		&$0.25 + 0.24$	&$0.44 + 0.40$    \\
    \midrule
    s=0.5, c=0.5, b=0.5        &$0.50$    &$0.99$	&$83.81 + 12.09$	&$0.25 + 0.15$	&$0.19 + 0.10$		&$0.28 + 0.23$	&$0.32 + 0.25$    \\
    s=0.5, c=0.5, b=0.5        &$0.60$    &$0.99$	&$89.80 + 11.95$	&$0.25 + 0.15$	&$0.20 + 0.10$		&$0.27 + 0.24$	&$0.34 + 0.26$    \\
    s=0.5, c=0.5, b=0.5        &$0.70$    &$0.99$	&$92.75 + 11.41$	&$0.26 + 0.16$	&$0.21 + 0.10$		&$0.26 + 0.24$	&$0.36 + 0.28$    \\
    s=0.5, c=0.5, b=0.5        &$0.80$    &$0.99$	&$94.58 + 11.04$	&$0.26 + 0.16$	&$0.21 + 0.10$		&$0.26 + 0.23$	&$0.37 + 0.28$    \\
    s=0.5, c=0.5, b=0.5        &$0.90$    &$0.99$	&$95.37 + 10.85$	&$0.27 + 0.16$	&$0.22 + 0.11$		&$0.25 + 0.23$	&$0.38 + 0.29$    \\
    s=0.5, c=0.5, b=0.5        &$0.99$    &$0.99$	&$95.72 + 10.69$	&$0.27 + 0.17$	&$0.23 + 0.11$		&$0.25 + 0.24$	&$0.39 + 0.30$    \\
    \midrule
    s=0.5, c=0.5, b=1.0        &$0.50$    &$0.99$	&$79.44 + 15.79$	&$0.25 + 0.14$	&$0.19 + 0.09$		&$0.27 + 0.26$	&$0.30 + 0.26$    \\
    s=0.5, c=0.5, b=1.0        &$0.60$    &$0.99$	&$86.74 + 16.18$	&$0.26 + 0.15$	&$0.20 + 0.09$		&$0.25 + 0.25$	&$0.34 + 0.29$    \\
    s=0.5, c=0.5, b=1.0        &$0.70$    &$0.99$	&$90.68 + 15.60$	&$0.27 + 0.16$	&$0.21 + 0.09$		&$0.25 + 0.23$	&$0.37 + 0.32$    \\
    s=0.5, c=0.5, b=1.0        &$0.80$    &$0.99$	&$92.80 + 15.33$	&$0.28 + 0.16$	&$0.22 + 0.10$		&$0.24 + 0.22$	&$0.41 + 0.37$    \\
    s=0.5, c=0.5, b=1.0        &$0.90$    &$0.99$	&$93.54 + 15.10$	&$0.28 + 0.17$	&$0.24 + 0.10$		&$0.24 + 0.21$	&$0.44 + 0.40$    \\
    s=0.5, c=0.5, b=1.0        &$0.99$    &$0.99$	&$93.79 + 14.78$	&$0.29 + 0.17$	&$0.25 + 0.10$		&$0.23 + 0.20$	&$0.46 + 0.41$    \\
    \bottomrule
  \end{tabular}
\end{table*}

\begin{table*}[!htbp]
  \caption{Comparison validity, sparsity, in-distributioness for finer ranges of target (unbalanced dataset, untrained encoder).}
  \label{tab:comparison_soft_targets_fine}
  \centering
  
  \begin{tabular}{llllllll}
    \toprule
                                &\multicolumn{2}{c}{Prob}         &\multicolumn{5}{c}{\textbf{Metrics}} \\
                               \cmidrule(r){2-3}                  \cmidrule(r){4-8} 
    \textbf{Method}            &\textbf{Min}   &\textbf{Max}      &\textbf{Validity}(\%)  &\boldsymbol{$L_{0}$}  &\boldsymbol{$L_{1}$}  &\boldsymbol{$MMD_{0}$}   &\boldsymbol{$MMD_{1}$} \\
    \midrule
    s=0.3, c=0.5, b=0.5        &$0.50$    &$0.60$	&$67.16 + 15.60	$    &$0.28 + 0.16$	    &$0.19 + 0.12$	    &$0.34 + 0.27$	    &$0.30 + 0.29$ \\
    s=0.3, c=0.5, b=0.5        &$0.60$    &$0.70$	&$87.01 + 12.28$	 &$0.29 + 0.17$	    &$0.21 + 0.13$	    &$0.32 + 0.27$	    &$0.34 + 0.34$ \\
    s=0.3, c=0.5, b=0.5        &$0.70$    &$0.80$	&$94.45 + 6.49$	     &$0.30 + 0.17$	    &$0.22 + 0.13$	    &$0.29 + 0.25$	    &$0.38 + 0.37$ \\
    s=0.3, c=0.5, b=0.5        &$0.80$    &$0.90$	&$97.13 + 4.70$	     &$0.31 + 0.18$	    &$0.24 + 0.13$	    &$0.25 + 0.24$	    &$0.41 + 0.40$ \\
    s=0.3, c=0.5, b=0.5        &$0.90$    &$0.99$	&$97.84 + 4.42$	     &$0.32 + 0.19$	    &$0.26 + 0.13$	    &$0.23 + 0.23$	    &$0.44 + 0.44$ \\
    \midrule
    s=0.4, c=0.5, b=0.5        &$0.50$    &$0.60$	&$62.88 + 16.07$	 &$0.25 + 0.15$	    &$0.17 + 0.10$	    &$0.34 + 0.26$	    &$0.32 + 0.31$ \\
    s=0.4, c=0.5, b=0.5        &$0.60$    &$0.70$	&$84.84 + 12.62$   	 &$0.26 + 0.16$	    &$0.19 + 0.11$	    &$0.32 + 0.26$	    &$0.36 + 0.33$ \\
    s=0.4, c=0.5, b=0.5        &$0.70$    &$0.80$	&$92.62 + 9.96$		 &$0.27 + 0.16$	    &$0.20 + 0.11$	    &$0.30 + 0.25$	    &$0.39 + 0.37$ \\
    s=0.4, c=0.5, b=0.5        &$0.80$    &$0.90$	&$95.44 + 9.45$    	 &$0.28 + 0.17$	    &$0.22 + 0.11$	    &$0.27 + 0.25$	    &$0.41 + 0.38$ \\
    s=0.4, c=0.5, b=0.5        &$0.90$    &$0.99$	&$96.15 + 9.07$ 	 &$0.29 + 0.18$	    &$0.23 + 0.11$	    &$0.25 + 0.24$	    &$0.43 + 0.39$ \\
    \midrule
    s=0.5, c=0.5, b=0.5        &$0.50$    &$0.60$	&$61.64 + 17.30$	 &$0.22 + 0.13$	    &$0.16 + 0.09$	    &$0.34 + 0.25$	    &$0.32 + 0.26$ \\
    s=0.5, c=0.5, b=0.5        &$0.60$    &$0.70$	&$80.91 + 17.18$	 &$0.24 + 0.14$	    &$0.17 + 0.10$	    &$0.31 + 0.25$	    &$0.33 + 0.26$ \\
    s=0.5, c=0.5, b=0.5        &$0.70$    &$0.80$	&$89.52 + 13.15$	 &$0.25 + 0.15$	    &$0.19 + 0.10$	    &$0.29 + 0.25$	    &$0.35 + 0.27$ \\
    s=0.5, c=0.5, b=0.5        &$0.80$    &$0.90$	&$93.91 + 11.30$	 &$0.26 + 0.16$	    &$0.21 + 0.10$	    &$0.27 + 0.23$	    &$0.37 + 0.29$ \\
    s=0.5, c=0.5, b=0.5        &$0.90$    &$0.99$	&$95.37 + 10.85$	 &$0.27 + 0.16$	    &$0.22 + 0.11$	    &$0.25 + 0.23$	    &$0.38 + 0.29$ \\
    \midrule
    s=0.5, c=0.5, b=1.0        &$0.50$    &$0.60$	&$52.48 + 19.11$	 &$0.22 + 0.13$	    &$0.13 + 0.06$ 	    &$0.36 + 0.29$	    &$0.31 + 0.24$ \\
    s=0.5, c=0.5, b=1.0        &$0.60$    &$0.70$	&$74.91 + 20.42$	 &$0.23 + 0.13$	    &$0.16 + 0.08$	    &$0.32 + 0.27$	    &$0.32 + 0.27$ \\
    s=0.5, c=0.5, b=1.0        &$0.70$    &$0.80$	&$86.58 + 17.45$	 &$0.25 + 0.15$	    &$0.18 + 0.09$	    &$0.28 + 0.25$	    &$0.35 + 0.29$ \\
    s=0.5, c=0.5, b=1.0        &$0.80$    &$0.90$	&$92.15 + 15.61$	 &$0.27 + 0.16$	    &$0.21 + 0.09$	    &$0.25 + 0.23$	    &$0.39 + 0.35$ \\
    s=0.5, c=0.5, b=1.0        &$0.90$    &$0.99$	&$93.54 + 15.10$	 &$0.28 + 0.17$	    &$0.24 + 0.10$	    &$0.24 + 0.21$	    &$0.44 + 0.40$ \\
    \bottomrule
  \end{tabular}
\end{table*}
