# Supplementary material for: Model-agnostic and Scalable Counterfactual Explanations via Reinforcement Learning
Source: arXiv:2106.02597 source file (2021-06-04)
Supplement: Supplementary file 4 [file 02-image_autoencoder.tex]

\subsection{Image autoencoders}

The MNIST encoder projects the input instances to a latent representation of dimension 32. We trained the autoencoder for 50K iteration with a batch size of 64, optimizing the Binary Cross-Entropy (BCE) using Adam optimizer\cite{kingma2014adam} with a learning rate of 1e-3. The CELEBA encoder projects the input space from 128x128 to a 128 embedding representation. We trained autoencoder for 350K iterations with a batch size of 128, optimizing the Mean Squared Error(MSE) using Adam optimizer\cite{kingma2014adam} with a learning rate of 1e-4.  Tables \ref{tab:image_autoenc_arch}, \ref{tab:image_blocks_arch} summarize the autoencoders's architecture for both datasets.

%% image autoencoder architecture
\begin{table*}
  \caption{Image autoencoders' architectures.}
  \label{tab:image_autoenc_arch}
  \centering
  
  \begin{tabular}{ll}
    \toprule
    \multicolumn{2}{c}{\textbf{Datasets}} \\
    \cmidrule(r){0-1} 
    \textbf{MNIST}         &\textbf{CELEBA}\\
    \midrule
    Conv2d(1, 16, kernel\_size=(3, 3), padding=1)  &ConvBlock(3, 32)\\
    MaxPool2d(kernel\_size=(2, 2), stride=2)       &ConvBlock(32, 64)\\
    Conv2d(16, 8, kernel\_size=(3, 3), padding=1)  &ConvBlock(64, 128\\
    MaxPool2d(kernel\_size=(2, 2), stride=2)       &ConvBlock(128, 256)\\
    Conv2d(8, 8, kernel\_size=(3, 3), padding=2)   &ConvBlock(256, 512)\\
    MaxPool2d(kernel\_size=(2, 2), stride=2)       &ConvBlock(512, 512)\\
    Flatten()                                      &Flatten()\\
    Linear(128, 32)                                &Linear(2048, 128)\\
    Tanh()                                         &Tanh()\\
    Linear(32, 128)                                &TransConvBlock(512, 512)\\
    Conv2d(8, 8, kernel\_size=(3, 3), padding=1)   &TansConvBlock(512, 512) \\
    Upsample(scale\_factor=2)                      &TransConvBlock(512, 256)\\
    Conv2d(8, 8, kernel\_size=(3, 3), padding=1)   &TransConvBlock(256, 128) \\
    Upsample(scale\_factor=2)                      &TransConvBlock(128, 64) \\
    Conv2d(8, 16, kernel\_size=(3, 3))             &TransConvBlock(64, 32) \\
    Upsample(scale\_factor=2)                      &TransConvBlock(32, 32) \\
    Conv2d(16, 1, kernel\_size=(3, 3), padding=1)  &TransConvBlock(32, 3) \\
     -                                             &Tanh()\\
    \bottomrule
  \end{tabular}
\end{table*}

%% blocks' architecture
\begin{table*}
  \caption{Blocks' architectures.}
  \label{tab:image_blocks_arch}
  \centering
  
  \begin{tabular}{p{5cm}p{5cm}}
    \toprule
    \multicolumn{2}{c}{\textbf{Blocks}} \\
    \cmidrule(r){0-1} 
    \textbf{ConvBlock}         &\textbf{TransConvBlock}\\
    \midrule
    Conv2d(in\_channels, out\_channels, kernel\_size=3, stride=2, padding=1)        &ConvTranspose2d(in\_channels, out\_channels, kernel\_size=3, stride=2, padding=1, output\_padding=1) \\
    BatchNorm2d(out\_channles)                                                      &BatchNorm2d(out\_channles) \\
    LeakyReLU()                                                                     &LeakyReLU() \\
    \bottomrule
  \end{tabular}
\end{table*}
