# Supplementary material for: Model-agnostic and Scalable Counterfactual Explanations via Reinforcement Learning
Source: arXiv:2106.02597 source file (2021-06-04)
Supplement: Supplementary file 7 [file 05-mmd_covertype.tex]

\subsection{In-distributionness results for Covertype dataset.}
\begin{table*}
  \caption{Covertype MMD}      
  \label{tab:mmd_covertype}
  \centering
  
  \resizebox{\textwidth}{!}{
  \begin{tabular}{llllllll}
    \toprule
    &               \multicolumn{7}{c}{\textbf{MMD per class} (1e-1)} \\
                    \cmidrule(r){2-8} 
    \textbf{Method}                 &\textbf{0}       &\textbf{1}       &\textbf{2}         &\textbf{3}         &\textbf{4}         &\textbf{5}         &\textbf{6}             \\
    \midrule
    LORE                            &$0.02\pm0.01$    &$0.11\pm0.05$    &$0.38\pm0.06$      &$1.47\pm0.33$      &$0.09\pm0.04$      &$0.57\pm0.05$      &$0.23\pm0.06$ \\
    \midrule
    MO	                            &$0.01\pm0.00$    &$0.09\pm0.03$    &$0.48\pm0.07$      &$1.21\pm0.11$      &$0.02\pm0.02$      &$0.61\pm0.10$      &$0.10\pm0.04$ \\
    \midrule
    DICE(random)	                &$0.17\pm0.06$    &$0.15\pm0.07$    &$0.94\pm0.72$      &$0.65\pm0.51$      &$0.63\pm0.47$      &$0.87\pm0.18$      &$0.36\pm0.13$ \\
    DICE(genetic)	                &$0.24\pm0.10$    &$0.07\pm0.07$    &$0.41\pm0.28$	    &$0.59\pm0.28$      &$0.38\pm0.17$      &$0.71\pm0.34$      &$0.44\pm0.20$ \\
    \midrule
    DiCE(bin, random)               &$0.17\pm0.06$    &$0.15\pm0.07$    &$0.94\pm0.72$	    &$0.65\pm0.51$      &$0.63\pm0.47$      &$0.87\pm0.18$	    &$0.36\pm0.13$ \\
    DiCE(bin, genetic)              &$0.27\pm0.10$    &$0.07\pm0.07$    &$0.47\pm0.26$      &$0.54\pm0.27$      &$0.36\pm0.18$      &$0.72\pm0.33$      &$0.46\pm0.20$ \\
    \midrule
    Ours(w/o AE)                    &$0.33\pm0.40$    &$0.33\pm0.18$    &$0.65\pm0.25$      &$1.04\pm0.51$      &$0.82\pm0.58$      &$0.78\pm0.31$      &$0.57\pm0.41$  \\
    Ours(w/o AE, cond)              &$0.25\pm0.20$    &$0.15\pm0.10$    &$0.49\pm0.26$      &$0.75\pm0.52$	    &$0.37\pm0.18$      &$0.52\pm0.34$      &$0.23\pm0.13$  \\
    \midrule
    Ours                            &$0.06\pm0.04$	  &$0.10\pm0.04$    &$0.32\pm0.25$	    &$1.47\pm0.44$      &$0.32\pm0.17$      &$0.82\pm0.25$	    &$0.17\pm0.11$ \\
    Ours(cond)                      &$0.04\pm0.02$    &$0.10\pm0.04$    &$0.25\pm0.08$      &$1.48\pm0.33$      &$0.18\pm0.10$      &$0.58\pm0.15$      &$0.12\pm0.09$ \\
    \bottomrule
  \end{tabular}
  }
\end{table*}
