# Supplementary material for: Model-agnostic and Scalable Counterfactual Explanations via Reinforcement Learning
Source: arXiv:2106.02597 source file (2021-06-04)
Supplement: Supplementary file 8 [file 06-samples_adult.tex]

\begin{figure*}
    \centering
    \includegraphics[width=\textwidth]{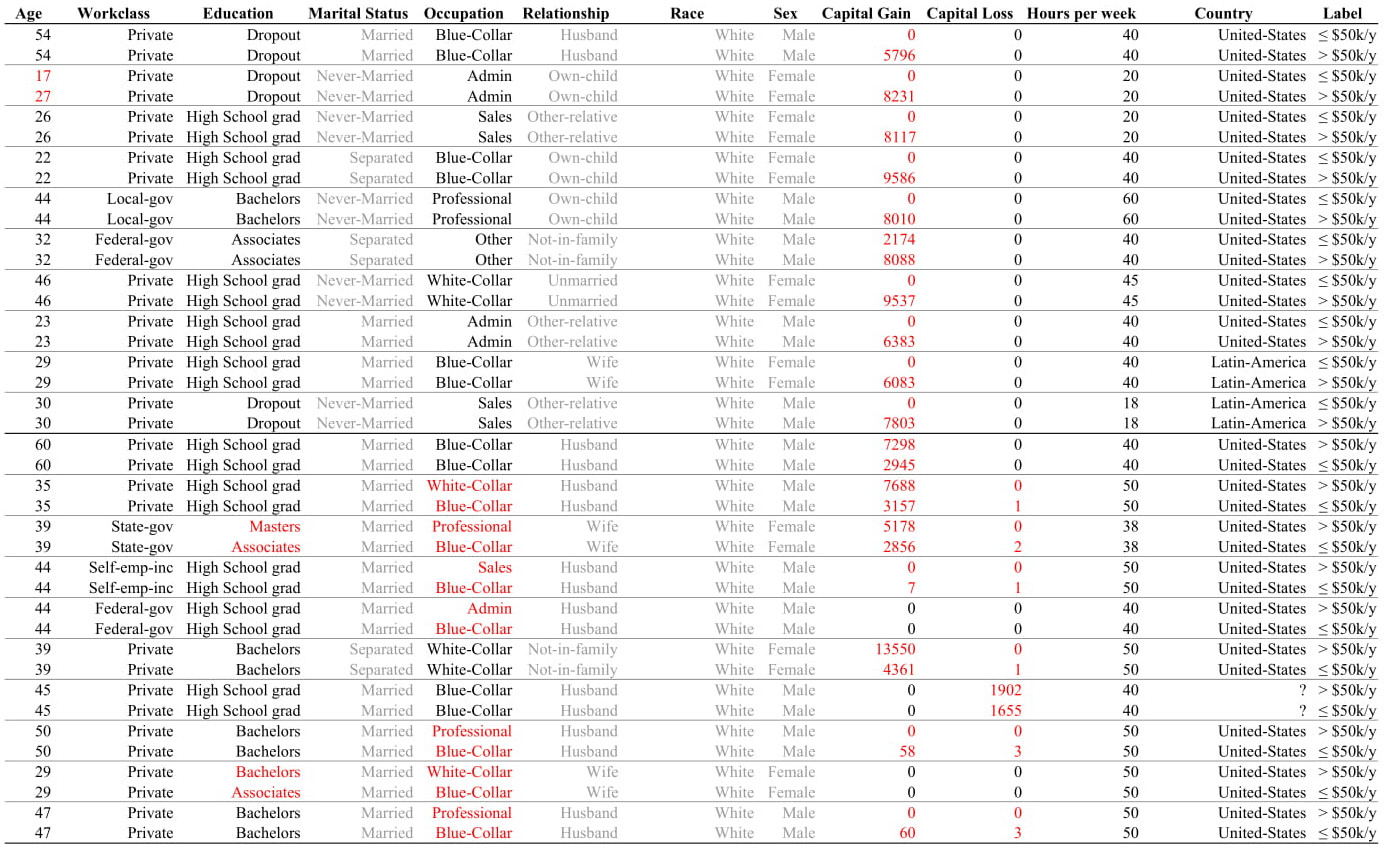}
    \caption{Unconditional counterfactuals Adult dataset.}
    \label{fig:my_label}
\end{figure*}

\begin{figure*}
    \centering
    \includegraphics[width=\textwidth]{imgs/tabular/adult/adult_uncond_cropped.jpg}
    \caption{Conditional counterfactuals Adult dataset.}
    \label{fig:my_label}
\end{figure*}
