# Supplementary material for: Model-agnostic and Scalable Counterfactual Explanations via Reinforcement Learning
Source: arXiv:2106.02597 source file (2021-06-04)
Supplement: Supplementary file 9 [file 07-samples_celeba.tex]

\pagebreak
\subsection{Samples CELEBA}

\begin{figure*}
    \centering
    \includegraphics[height=0.95\textheight]{imgs/celeba/one2all/with_spacing.png}
    \caption{One instance to all classes on CELEBA dataset.}
    \label{fig:mnist_samples}
\end{figure*}
