# Supplementary material for: Model-agnostic and Scalable Counterfactual Explanations via Reinforcement Learning
Source: arXiv:2106.02597 source file (2021-06-04)
Supplement: Supplementary file 10 [file 08-samples_mnist.tex]

\clearpage
\subsection{Samples MNIST}

\begin{figure*}
    \centering
    \includegraphics[width=1.0\textwidth]{imgs/mnist/one2all/with_spacing.png}
    \caption{One instance to all classes on MNIST dataset.}
    \label{fig:mnist_samples}
\end{figure*}
